# Supplementary material for: Unitary coupled-cluster based self-consistent polarization propagator theory: a quadratic unitary coupled-cluster singles and doubles scheme
Source: arXiv:2107.01099 source file (2021-09-23)
Supplement: Supplementary file 1 [file SI.pdf]

**Supplementary Information for “Unitary coupled-cluster based self-consistent polarization propagator theory: a quadratic unitary coupled-cluster singles and doubles scheme”**

## A conical intersection in FOH

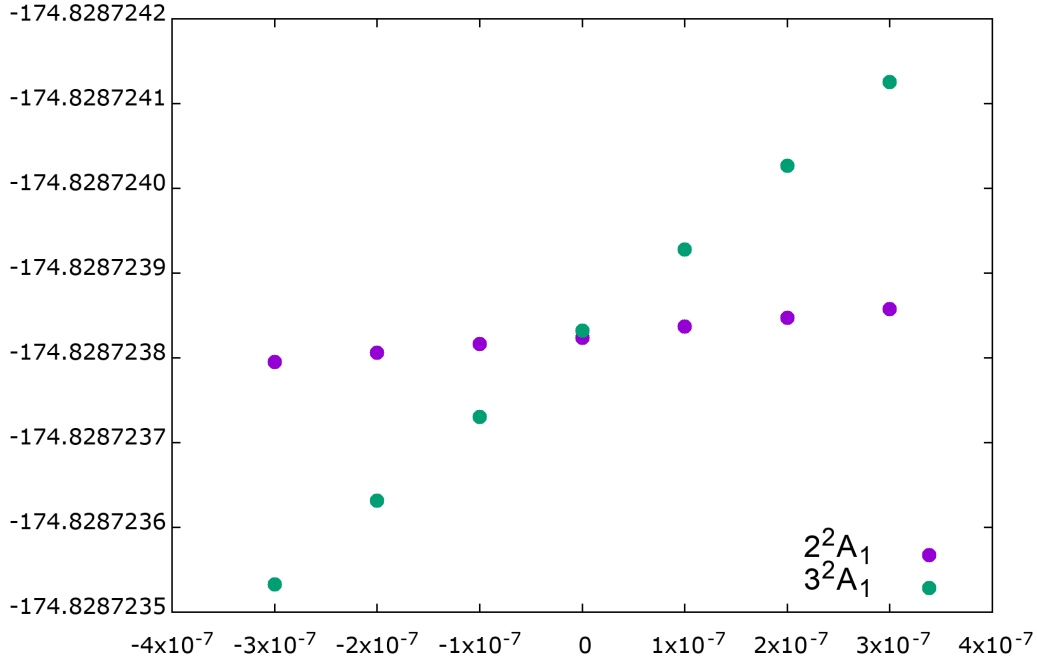

FIG. 1. The potential energy surfaces of FOH around an intersecting point ( $R_{FO}=1.2924959$  Å,  $R_{OH}=1.0902915$  Å,  $\angle_{H-O-F}=91.112557^\circ$ ) between the  $2^1A_1$  and  $3^1A_1$  states computed at the qUCCSD/aug-cc-pVDZ level with all electron correlated. The x axis is the displacement of  $R_{FO}$  in Å, and the y axis is the electronic energies in Hartree.

Although general characterization of same-symmetry conical intersections using qUCCSD will have to wait for the implementation of analytic gradients and derivative coupling, it is worthwhile mentioning that the hermitian nature of qUCCSD enables the description of degeneracies between electronic states. As an example, we have enclosed in Figure 1 qUCCSD calculations of potential energy surfaces in the immediate vicinity of one of the conical intersection point between the  $2^1A_1$  and  $3^1A_1$  states of the FOH molecule. The qUCCSD calculations show the correct degeneracy at the intersecting point and the correct linear behavior of the electronic energies with respect to the displacements. In contrast, EOM-CCSD calculations produce complex eigenvalues when the energies of these two state are within 0.03 eV of each other.
